# Supplementary material for: Effects of Non-local Pseudopotentials on the Electrical and Thermal Transport Properties of Aluminum: A Density Functional Theory Study
Source: arXiv:2402.15706 source file (2024-02-24)
Supplement: Supplementary file 1 [file SM.pdf]

# Supplementary Material: Effects of Non-local Pseudopotentials on the Electrical and Thermal Transport Properties of Aluminum: A Density Functional Theory Study

Qianrui Liu (刘千锐) and Mohan Chen (陈默涵)

TABLE I. Fitting parameters for conductivities of aluminum at a density of 2.35 g/cm$^3$ and various temperatures $T$. The fitting range is represented by $\omega_1$ and $\omega_2$. $\sigma$ denotes the DC electrical conductivity, while $\tau$ corresponds to the relaxation time. $\kappa$ represents the thermal conductivity and $a$,$b$, and $c$ are fitting parameters of the thermal conductivities.

| $T$ (eV) | $\omega_1$ (eV) | $\omega_2$ (eV) | $\sigma$ ($10^6$Sm$^{-1}$) | $\tau$ (eV$^{-1}$) | $\kappa$ ($10^3$Wm$^{-1}$K$^{-1}$) | $a$ (eV$^{-2}$) | $b$ (eV$^{-4}$) | $c$ (eV$^{-6}$) |
|---|---|---|---|---|---|---|---|---|
| 0.086 | 0.15 | 1 | 3.892 | 1.689 | 0.096 | 14.408 | - | - |
| 0.2 | 0.15 | 1.15 | 2.892 | 1.223 | 0.160 | 0.8456 | -0.46472 | 0.140056 |
| 0.5 | 0.15 | 1.15 | 2.119 | 0.884 | 0.304 | 0.6901 | 0.00371 | -0.031406 |
| 1 | 0.15 | 1.55 | 1.733 | 0.711 | 0.478 | 0.5248 | -0.02974 | 0.004622 |
| 1.5 | 0.15 | 1.95 | 1.568 | 0.630 | 0.617 | 0.3928 | -0.00930 | 0.001265 |
| 2 | 0.15 | 2.15 | 1.481 | 0.588 | 0.740 | 0.3240 | 0.00073 | -0.000374 |
| 3 | 0.15 | 2.15 | 1.274 | 0.491 | 0.852 | 0.2035 | -0.00114 | 0.000064 |
| 5 | 0.15 | 3.15 | 1.014 | 0.369 | 0.959 | 0.0778 | 0.00270 | -0.000137 |
| 8 | 0.15 | 4.15 | 0.821 | 0.286 | 1.210 | 0.0430 | 0.00111 | -0.000025 |
| 10 | 0.15 | 5.15 | 0.738 | 0.247 | 1.399 | 0.0344 | 0.00085 | -0.000015 |

## I. FITTING RESULTS

In this study, we employ specific functions to fit the electrical and thermal conductivities at small frequencies in order to estimate their values at zero frequency. The fitting ranges for each conductivity are summarized in Table I. To fit the electronic conductivity, we utilize a Drude function [1] given by:

$$\sigma(\omega) = \frac{\sigma}{1+\omega^2\tau^2}, \tag{1}$$

where $\tau$ represents the relaxation time to be determined through fitting, and $\sigma$ corresponds to the DC electrical conductivity. For the thermal conductivity, we treat the results obtained at 1000 K and other temperatures separately. In the case of 1000 K, a linear function is employed:

$$\kappa(\omega) = \kappa + a\omega. \tag{2}$$

On the other hand, at high temperatures, a more complex function is used:

$$\kappa(\omega) = \frac{\kappa}{1+a\omega^2+b\omega^4+c\omega^6}, \tag{3}$$

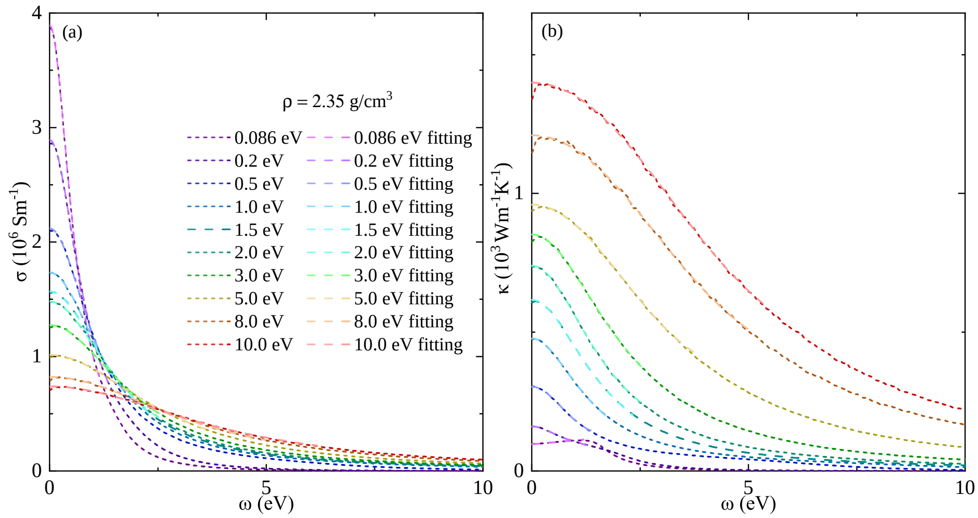


FIG. 1. Dynamic (a) electrical and (b) thermal conductivities of liquid and warm dense aluminum at a density of 2.35 g/cm$^3$ and temperatures ranging from 0.086 to 10 eV. Short dash lines represent the computational results, while normal dash lines indicate the fitted results. The cell contains 256 atoms for temperatures up to 5 eV and 108 atoms for higher temperatures. Pseudopotential NC11 is utilized with non-local potential corrections.

where $a$, $b$, and $c$ are parameters to be determined through fitting. The fitting results can be found in Tables I and II. Fig. 1 and 2 illustrate the dynamic results of aluminum at densities of aluminum at the density of 2.35 g/cm$^3$ and 2.70 g/cm$^3$, separately. These figures exhibit the excellent performance of these fitting methods in capturing the electrical and thermal conductivities.

## II. TEMPERATURE DEPENDENT XC

Additionally, we utilize a temperature-dependent exchange-correlation (XC) functional called KSDT to compute the electrical and thermal conductivities. The corresponding results are presented in Fig. 3. It is evident that the choice of XC functional does not significantly impact the results for densities of 2.35 and 2.70 g/cm$^3$, as well as temperatures ranging from 0.2 to 10 eV.

TABLE II. Dynamic (a) electrical and (b) thermal conductivities of liquid and warm dense aluminum at a density of 2.70 g/cm$^3$ and temperatures ranging from 0.086 to 10 eV. Short dash lines represent the computational results, while normal dash lines indicate the fitted results. The cell contains 256 atoms for temperatures up to 5 eV and 108 atoms for higher temperatures. Pseudopotential NC11 is utilized with non-local potential corrections.

| $T$ (eV) | $\omega_1$ (eV) | $\omega_2$ (eV) | $\sigma$ ($10^6$Sm$^{-1}$) | $\tau$ (eV$^{-1}$) | $\kappa$ ($10^3$Wm$^{-1}$K$^{-1}$) | $a$ (eV$^{-2}$) | $b$ (eV$^{-4}$) | $c$ (eV$^{-6}$) |
|---|---|---|---|---|---|---|---|---|
| 0.2 | 0.15 | 1.15 | 3.464 | 1.267 | 0.192 | 0.9884 | -0.58912 | 0.182928 |
| 0.5 | 0.15 | 1.15 | 2.547 | 0.925 | 0.368 | 0.7986 | -0.05273 | -0.012107 |
| 1 | 0.15 | 1.55 | 2.158 | 0.773 | 0.614 | 0.6877 | -0.04692 | 0.005068 |
| 1.5 | 0.15 | 1.95 | 1.881 | 0.667 | 0.757 | 0.4861 | -0.01994 | 0.002021 |
| 2 | 0.15 | 2.15 | 1.755 | 0.616 | 0.884 | 0.3943 | -0.01831 | 0.001948 |
| 3 | 0.15 | 2.15 | 1.521 | 0.518 | 1.011 | 0.2451 | -0.01171 | 0.001479 |
| 5 | 0.15 | 3.15 | 1.191 | 0.391 | 1.115 | 0.1007 | 0.00070 | -0.000059 |
| 8 | 0.15 | 4.15 | 0.949 | 0.296 | 1.364 | 0.0497 | 0.00078 | -0.000027 |
| 10 | 0.15 | 5.15 | 0.821 | 0.245 | 1.536 | 0.0314 | 0.00108 | -0.000024 |

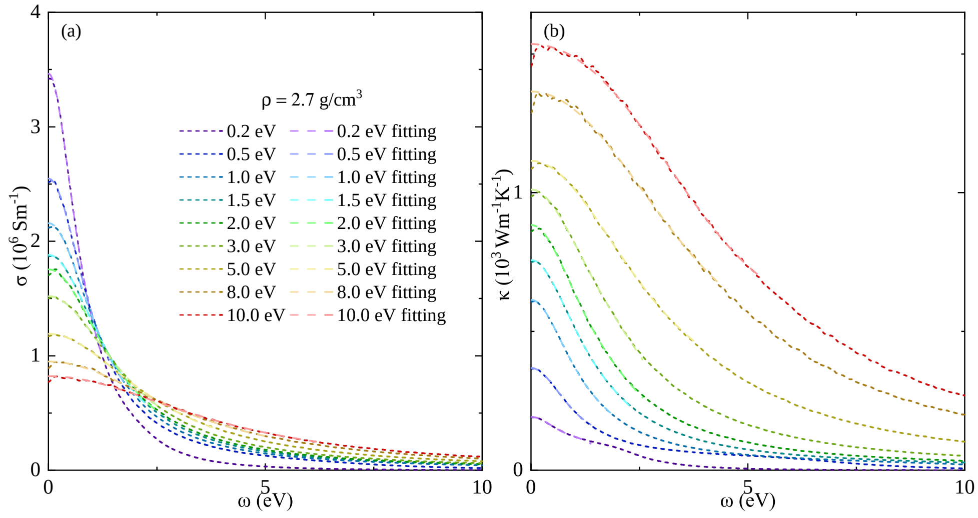


FIG. 2. Fitting parameters for conductivities of aluminum at a density of 2.70 g/cm$^3$ and various temperatures $T$. The fitting range is represented by $\omega_1$ and $\omega_2$. $\sigma$ denotes the DC electrical conductivity, while $\tau$ corresponds to the relaxation time. $\kappa$ represents the thermal conductivity and $a$,$b$, and $c$ are fitting parameters of the thermal conductivities.

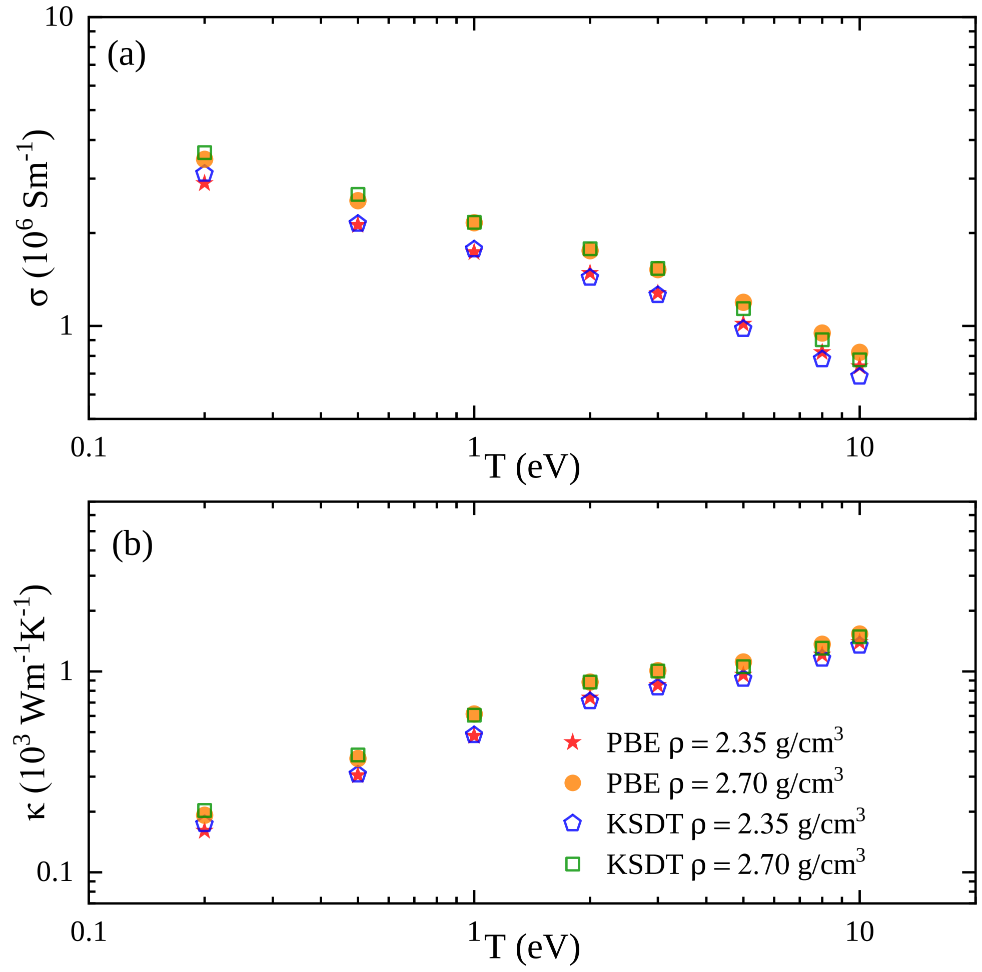


FIG. 3. (a)Electrical and (b)thermal conductivities of aluminum ranging from 0.2 eV to 10 eV. The results are presented for densities of 2.35 and 2.70 g/cm$^3$. Hollow symbols in the graph represent results obtained using the KSDT method, while solid symbols represent results obtained using the PBE method.

## III. CONDUCTIVITY DATA

All results are listed in Table III - VI for ease of reference.

TABLE III. Electrical conductivities ($10^6$Sm$^{-1}$) of aluminum at densities of 2.35 g/cm$^3$ and various temperatures $T$.

| $T$ (eV) | 0.086 | 0.2 | 0.5 | 1.0 | 1.5 | 2.0 | 3.0 | 5.0 | 8.0 | 10.0 |
|---|---|---|---|---|---|---|---|---|---|---|
| NC3 | 5.298 | 3.926 | 2.868 | 2.343 | 2.114 | 1.986 | 1.689 | 1.329 | 1.118 | 1.056 |
| NC11 | 5.450 | 4.033 | 2.934 | 2.380 | 2.127 | 1.974 | 1.624 | 1.187 | 0.886 | 0.768 |
| NC3 corr. | 4.124 | 3.024 | 2.178 | 1.748 | 1.556 | 1.446 | 1.192 | 0.894 | 0.727 | 0.689 |
| NC11 corr. | 3.892 | 2.892 | 2.119 | 1.733 | 1.568 | 1.481 | 1.274 | 1.014 | 0.821 | 0.738 |
| NC11 KSDT | - | 3.106 | 2.141 | 1.768 | - | 1.429 | 1.256 | 0.976 | 0.778 | 0.685 |

TABLE IV. Thermal conductivities ($10^3$Wm$^{-1}$K$^{-1}$) of aluminum at densities of 2.35 g/cm$^3$ and various temperatures $T$.

| $T$ (eV) | 0.086 | 0.2 | 0.5 | 1.0 | 1.5 | 2.0 | 3.0 | 5.0 | 8.0 | 10.0 |
|---|---|---|---|---|---|---|---|---|---|---|
| NC3 | 0.131 | 0.218 | 0.411 | 0.646 | 0.829 | 0.992 | 1.147 | 1.412 | 2.050 | 2.600 |
| NC11 | 0.135 | 0.224 | 0.421 | 0.651 | 0.819 | 0.963 | 1.070 | 1.141 | 1.367 | 1.543 |
| NC3 corr. | 0.102 | 0.168 | 0.312 | 0.481 | 0.607 | 0.718 | 0.810 | 0.963 | 1.452 | 1.941 |
| NC11 corr. | 0.096 | 0.160 | 0.304 | 0.478 | 0.617 | 0.740 | 0.852 | 0.959 | 1.210 | 1.399 |
| NC11 KSDT | - | 0.173 | 0.306 | 0.480 | - | 0.709 | 0.831 | 0.918 | 1.155 | 1.341 |

TABLE V. Electrical conductivities ($10^6$Sm$^{-1}$) of aluminum at densities of 2.70 g/cm$^3$ and various temperatures $T$.

| $T$ (eV) | 0.2 | 0.5 | 1.0 | 1.5 | 2.0 | 3.0 | 5.0 | 8.0 | 10.0 |
|---|---|---|---|---|---|---|---|---|---|
| NC3 | 4.695 | 3.446 | 2.923 | 2.546 | 2.368 | 2.033 | 1.581 | 1.308 | 1.189 |
| NC11 | 4.674 | 3.431 | 2.896 | 2.507 | 2.308 | 1.931 | 1.408 | 1.034 | 0.862 |
| NC3 corr. | 3.508 | 2.536 | 2.116 | 1.814 | 1.665 | 1.393 | 1.032 | 0.827 | 0.748 |
| NC11 corr. | 3.464 | 2.547 | 2.158 | 1.881 | 1.755 | 1.521 | 1.191 | 0.949 | 0.821 |
| NC11 KSDT | 3.642 | 2.668 | 2.167 | - | 1.780 | 1.535 | 1.137 | 0.903 | 0.777 |

TABLE VI. Thermal conductivities ($10^3$Wm$^{-1}$K$^{-1}$) of aluminum at densities of 2.70 g/cm$^3$ and various temperatures $T$.

| $T$ (eV) | 0.2 | 0.5 | 1.0 | 1.5 | 2.0 | 3.0 | 5.0 | 8.0 | 10.0 |
|---|---|---|---|---|---|---|---|---|---|
| NC3 | 0.260 | 0.499 | 0.834 | 1.027 | 1.196 | 1.379 | 1.665 | 2.475 | 3.118 |
| NC11 | 0.259 | 0.497 | 0.826 | 1.004 | 1.148 | 1.275 | 1.339 | 1.554 | 1.711 |
| NC3 corr. | 0.194 | 0.368 | 0.605 | 0.733 | 0.840 | 0.948 | 1.101 | 1.727 | 2.306 |
| NC11 corr. | 0.192 | 0.368 | 0.614 | 0.757 | 0.884 | 1.011 | 1.115 | 1.364 | 1.536 |
| NC11 KSDT | 0.203 | 0.384 | 0.606 | - | 0.884 | 1.002 | 1.057 | 1.304 | 1.490 |

[1] M. P. Desjarlais, J. D. Kress, and L. A. Collins, Electrical conductivity for warm, dense aluminum plasmas and liquids, Phys. Rev. E **66**, 025401 (2002).
